# Supplementary material for: ELT: Elastic Looped Transformers for Visual Generation
Source: arXiv:2604.09168 source file (2026-07-23)
Supplement: Supplementary file 1 [file imp_supp.tex]

\begin{table}[htbp]
\centering
\small
\caption{\textbf{Configurations and Hyperparameters.} (a) Settings for Masked Generative Models across two datasets. (b) Settings for Diffusion Models.}
\label{tab:imp_supp}
\vspace{2mm}

\begin{tabular}{lcc}
\toprule
\multicolumn{3}{c}{\textbf{(a) Masked Generative Models}} \\
\midrule
Config & Imagenet $256\times256$ & UCF-101 \\
\midrule
Codebook Size & 1024 & 1024 \\
Embedding dim & 1024 & 1024 \\
Image size & 256 & 128 \\
Latent shape & (1, 16, 16) & (4, 16, 16) \\
\midrule
\# Epochs & 270 & 2000 \\
Batch Size & 512 & 256 \\
\% Training label drop & 10 & 0 \\
Student sampling dist. & Uniform & Uniform \\
\# Warmup Steps & 15k (linear) & 15k (linear) \\
Max learning rate & $10^{-4}$ & $10^{-4}$ \\
Learning rate schedule & Cosine & Cosine \\
Optimizer & AdamW & AdamW \\
($\beta_1, \beta_2$) & (0.9, 0.96) & (0.9, 0.96) \\
Weight decay & 4.5e-2 & 4.5e-2 \\
\midrule
\# Sampling Steps & 24 & 12 \& 24 \\
Masking Schedule & Cosine & Cosine \\
CFG & $\checkmark$ & $\times$ \\
Sampling temperature & (0.5, 0.8) & (0.5, 0.8) \\
\bottomrule
\end{tabular}

\vspace{6mm} % Space between the two sub-tables

\begin{tabular}{lc}
\toprule
\multicolumn{2}{c}{\textbf{(b) Diffusion Models}} \\
\midrule
\textbf{Config} & \textbf{Value} \\
\midrule
Hidden dim & 2048 \\
Head dim & 128 \\
Latent shape & (4, 32, 32) \\
MLP expansion & $4\times$ \\
Dropout & 0.1 \\
\midrule
\# Training Steps & 500K \\
Batch Size & 512 \\
\% Training Label drop & 10 \\
Student sampling dist. & Uniform \\
Learning rate & $10^{-4}$ \\
Warmup steps & 10K (linear) \\
Optimizer & AdamW \\
($\beta_1, \beta_2$) & (0.9, 0.99) \\
Weight decay & 0.01 \\
Gradient clipping & 1.0 ($L_2$) \\
EMA decay & 0.9999 \\
Noise Schedule & Cosine \\
Prediction & $v$-prediction \\
Loss Function  & SigmoidELBO \\
% Curriculum steps & 500K \\
Sampling steps & 512 \\
Sampler & DDPM ($\eta=0.3$) \\
CFG scale & 3.0 \\
\bottomrule
\end{tabular}
\end{table}
